# Supplementary material for: Exploiting Non-Abelian Point-Group Symmetry to Estimate the Exact Ground-State Correlation Energy of Benzene in a Polarized Split-Valence Triple-Zeta Basis Set
Source: arXiv:2407.21576 ancillary file (2024-07-31)
Supplement: Supplementary file 1 [file si.pdf]

# Supporting Information: Exploiting Non-Abelian Point-Group Symmetry to Estimate the Exact Ground-State Correlation Energy of Benzene in a Polarized Split-Valence Triple-Zeta Basis Set

Jonas Greiner,[†] Jürgen Gauss,[†] and Janus J. Eriksen[*,‡]

†*Department Chemie, Johannes Gutenberg-Universität Mainz*

*Duesbergweg 10–14, 55128 Mainz, Germany*

‡*DTU Chemistry, Technical University of Denmark*

*Kemitorvet Bldg. 206, 2800 Kgs. Lyngby, Denmark*

E-mail: janus@dtu.dk

# 1 List of Method Acronyms

Table S1: Acronyms of all methods referenced in the main study.

| Acronym | Method | References |
|---|---|---|
| CCSD | CC with S and D excitations | S1 |
| CCSD(T) | CCSD w/ perturbative T excitations | S2 |
| CCSDT | CC with S, D, and T excitations | S3–S5 |
| CCSDT(Q) | CCSDT w/ perturbative Q excitations | S6 |
| CCSDTQ | CC with S, D, T, and Q excitations | S7,S8 |
| $i$-FCIQMC | Initiator approximation to FCIQMC | S9,S10 |
| ASCI | Adaptive sampling CI | S11–S13 |
| SHCI | Semistochastic heat-bath CI | S14–S16 |
| iCI | Iterative CI with selection | S17–S20 |
| AS-FCIQMC | Adaptive-shift FCI quantum Monte Carlo | S21 |
| CAD-FCIQMC | Cluster-analysis-driven FCIQMC | S22–S25 |
| DMRG | Density matrix renormalization group | S26–S36 |
| MBE-FCI | Many-body expanded FCI | S37–S43 |
| FCCR | Full CC reduction | S44,S45 |
| AFQMC | Auxiliary-field quantum Monte Carlo | S46–S52 |
| CIPSI | CI perturbatively selected iteratively | S53–S55 |
| iFCI | Incremental FCI | S56–S59 |

# 2 Symmetry Exploitation

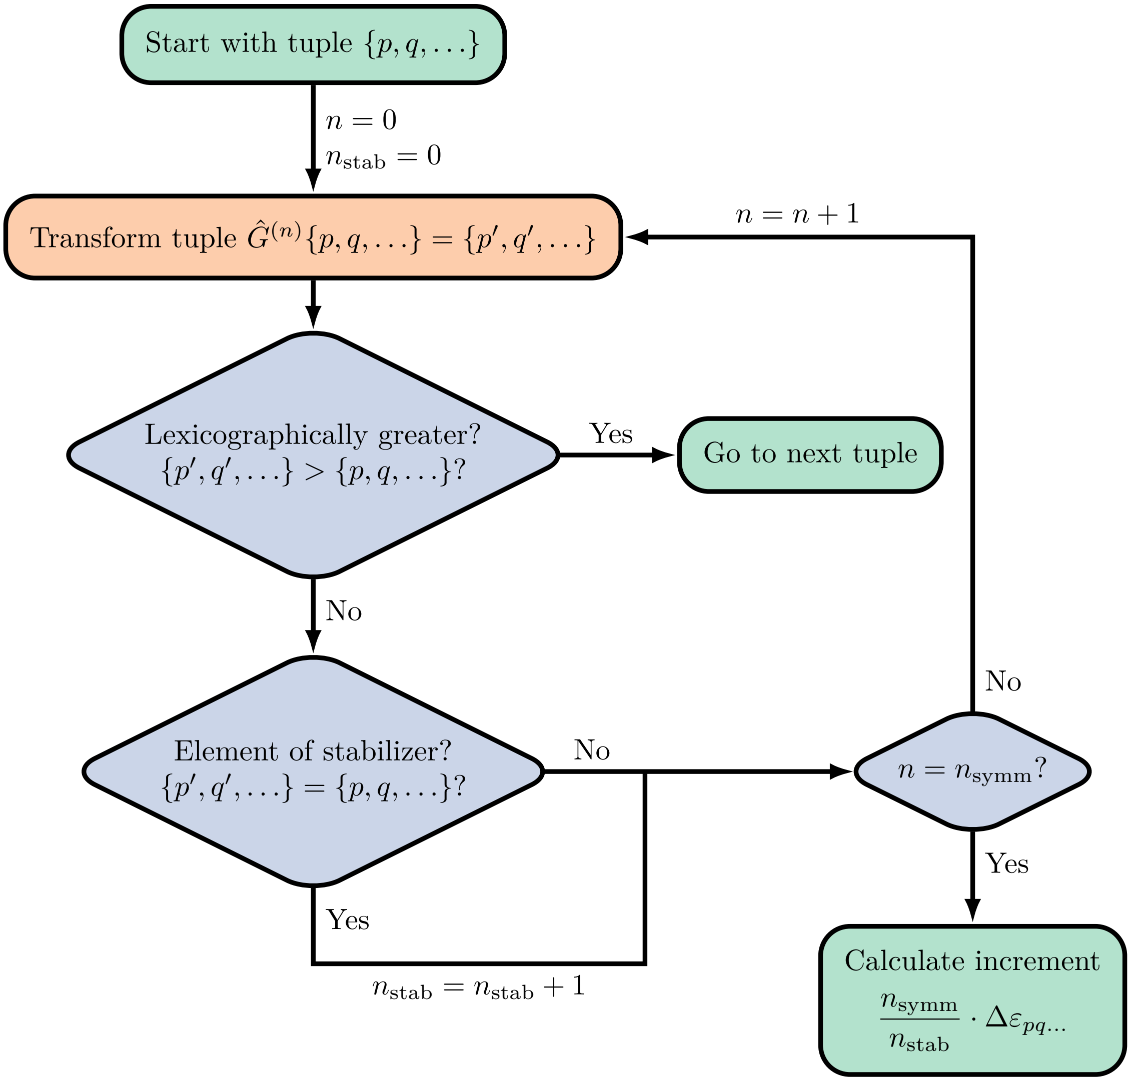


Figure S1: Flowchart for the *petite* list algorithm applied to MBE-FCI theory.

The schematic representation of the *petite* list algorithm is illustrated in Fig. S1. For every given orbital tuple, all symmetry operations of the molecular point group are applied. Whenever a transformed tuple is lexicographically greater than the original orbital tuple, the tuple is not symmetry-unique and will therefore be skipped. The order of the stabilizer is calculated while all symmetry operations are applied to determine the total cardinality of the symmetry-equivalent set upon identifying the symmetry-unique tuple in question.

# 3 Implementation

The application of MBE-FCI theory to larger systems necessitates a highly efficient implementation capable of exploiting the embarrassingly parallel nature of this method. Our `PyMBE` code works by dividing all necessary calculations at a given expansion order amongst all processes in a round-robin fashion.[S60] The tuples themselves are stored as hashes together with their corresponding increments in associative arrays on every node in shared memory, employing a hybrid MPI+MPI approach to memory allocation and access.[S61] This approach significantly reduces memory requirements while also limiting the amount of communication between processes. The total number of non-redundant increments has to be known before the shared memory can be allocated; for this reason, our algorithm first determines this number in a parallelized dry-run by looping over all possible tuples, applying all symmetry operations, and counting only those that are lexicographically greatest. The symmetry-unique increments are then calculated and stored in shared memory on all nodes.

# 4 Calibration

In Ref. S62, a reference space of six PM localized $\pi$-orbitals was used in the MBE-FCI calculation. The automatic reference space detection introduced in Ref. S43 comes to the same conclusion for a starting quantum fidelity threshold of 0.95 as the wave function character significantly changes upon adding these six $\pi$-orbitals. When a high-level CC base model is used (CCSDT or CCSDTQ), smaller reference spaces are feasible as the base model already approximately captures the correlation introduced by the $\pi$-orbitals. Nevertheless, calculations including sets of $\pi$-orbitals in the reference space may accelerate convergence of the MBE and should therefore be examined for accurate calculations of this system.

From this analysis, two options for the reference space emerge: (i) an empty reference space combined with a PM localized expansion space, and (ii) a reference space involving the

symmetry-equivalent set of three occupied $\pi$-orbitals and the symmetry-equivalent set of three virtual $\pi$-orbitals combined with the remaining PM LMOs in the expansion space. A third option (iii), an intermediately sized reference space, can be constructed by choosing the two sets of degenerate $\pi$-orbitals in the CMO basis and localizing the remaining orbitals to add these to the expansion space. While this procedure limits the localizability of the remaining $\pi$-orbitals, the ability of the delocalized basis to compress correlation into only four $\pi$-orbitals could be beneficial to reduce the size of the individual calculations. An equivalent approach, combining a delocalized reference space with a localized expansion space, was tested on smaller systems in Ref. S43 and is now applied to benzene in this work.

Realistically, individual increment calculations should not grow beyond an active space size of 14 electrons in 14 orbitals as the CI and sigma vectors become too large to be simultaneously stored in memory on nodes with a large number of cores. As a result, for two-orbital clusters in the expansion space, reference space (i) will be able to recover all contributions through MBE order 14, reference space (ii) will be able to recover all contributions through order 8, and reference space (iii) will be able to recover all contributions through order 10. Calculations based on reference spaces (ii) and (iii) will also describe higher-order contributions that involve the $\pi$-orbitals included in the respective reference spaces.

As a result of our clustering of expansion spaces, MBE-FCI calculations are typically no longer limited by an inability to perform an exceedingly large number of increment calculations. In fact, increment active spaces tend to grow too large before this point is met. For this reason, the benzene calculations considered herein have deliberately not been subject to any screening but instead manually truncated at a specified expansion order (cf. main study). Additionally, the error estimation technique proposed in Ref. S43 is currently not implemented for use in conjunction with CC base models and has thus not been applied.

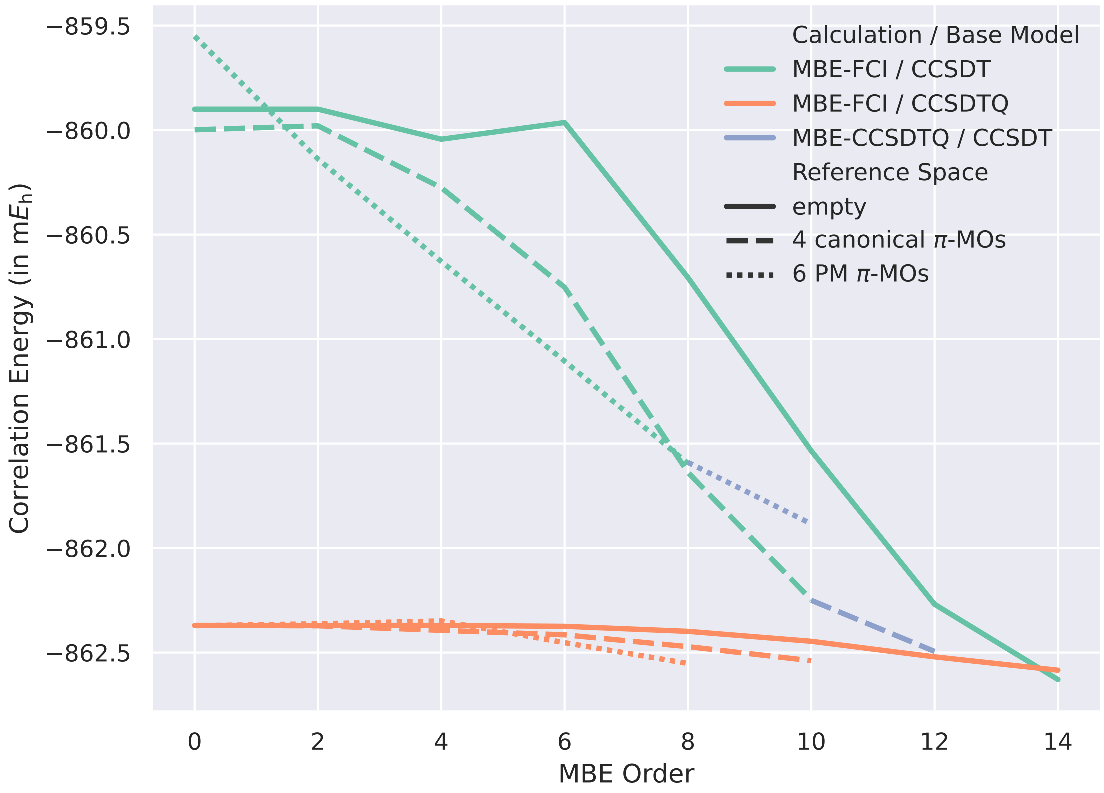


Figure S2: MBE-FCI/cc-pVDZ energy convergence for different choices of reference spaces and base models. Calculations that make use of a CCSDT base model are additionally augmented by an MBE-CCSDTQ/CCSDT residual result at the final MBE order.

Calculations involving the different reference space choices in conjunction with CCSDT and CCSDTQ base models are presented in Fig. S2. For these calculations, full $D_{6h}$ LMO point-group symmetry is exploited and clusters of orbital pairs have been constructed from early-order MBE-FCI information using the algorithm previously outlined in Ref. S43.

The calculations that make use of a CCSDT base model can be further improved by adding a residual MBE-CCSDTQ/CCSDT energy contribution at the final order. Regardless, the calculation based on all six PM $\pi$-orbitals in the reference space and the CCSDT base model is unable to converge before the calculation becomes too expensive. In general, calculations that involve larger reference spaces will converge quicker but are also limited by the size of the resulting increment active spaces. The calculation including four canonical $\pi$-orbitals in the

reference space, on the other hand, appears to strike a favorable balance between accelerated convergence (due to the inclusion of the most correlated $\pi$-orbitals in every individual increment calculation) and the limited increment active space size at the maximum MBE order.

All calculations employing a CCSDTQ base model add only a small correction to the initial CCSDTQ starting point, thus supporting the previous discussion in Ref. S62 on the ability of the CCSDTQ method to accurately describe this dynamically correlated system. In general, the contributions at early MBE orders for base model calculations will be small because the increment CASCC calculations are able to accurately describe small active spaces. At later MBE orders, the contributions will first increase and then decrease again as the MBE converges. Even if the MBE is terminated before convergence, all late-order contributions are recovered up to the base model level of theory. The empty reference space MBE-FCI/CCSDTQ calculation leads to a correlation energy of $-862.6$ m$E_\mathrm{h}$ which likely constitutes our current best estimate of the frozen-core correlation energy of benzene in a cc-pVDZ basis set. This estimate is arguably significantly more accurate than the MBE-FCI result in Ref. S62, both due to the inclusion of the CCSDTQ base model, but also the fact that all possible 7-orbital contributions are accounted for. In this calculation, all contributions are treated to infinite MBE order at the CCSDTQ level, while all contributions through order 14 are treated at the FCI level. At that order, the FCI correction to CCSDTQ is all but converged and future orders are expected to result in only a minor decrease of the correlation energy. Both results employing larger reference spaces agree with this prediction.

Treating benzene in a cc-pVTZ basis set, only calculations employing non-empty reference spaces are feasible. The corresponding empty reference space calculations would involve around 800M increments at MBE order 12 and 20B increments at MBE order 14 which becomes impractical both due to computational effort and numerical accuracy as the increment energies approach the convergence criterion of the CASCI calculations.

# References

(S1) Purvis, III, G. D.; Bartlett, R. J. A Full Coupled-Cluster Singles and Doubles Model: The Inclusion of Disconnected Triples. J. Chem. Phys. **1982**, 76, 1910.

(S2) Raghavachari, K.; Trucks, G. W.; Pople, J. A.; Head-Gordon, M. A Fifth-Order Perturbation Comparison of Electron Correlation Theories. Chem. Phys. Lett. **1989**, 157, 479.

(S3) Noga, J.; Bartlett, R. J. The Full CCSDT Model for Molecular Electronic Structure. J. Chem. Phys. **1987**, 86, 7041.

(S4) Noga, J.; Bartlett, R. J. Erratum: The Full CCSDT Model for Molecular Electronic Structure. J. Chem. Phys. **1988**, 89, 3401.

(S5) Scuseria, G. E.; Schaefer, III, H. F. A New Implementation of the Full CCSDT Model for Molecular Electronic Structure. Chem. Phys. Lett. **1988**, 152, 382.

(S6) Bomble, Y. J.; Stanton, J. F.; Kállay, M.; Gauss, J. Coupled-Cluster Methods Including Noniterative Corrections for Quadruple Excitations. J. Chem. Phys. **2005**, 123, 054101.

(S7) Oliphant, N.; Adamowicz, L. Coupled-Cluster Method Truncated at Quadruples. J. Chem. Phys. **1991**, 95, 6645.

(S8) Kucharski, S. A.; Bartlett, R. J. The Coupled-Cluster Single, Double, Triple, and Quadruple Excitation Method. J. Chem. Phys. **1992**, 97, 4282.

(S9) Cleland, D.; Booth, G. H.; Alavi, A. Communications: Survival of the Fittest: Accelerating Convergence in Full Configuration-Interaction Quantum Monte Carlo. J. Chem. Phys. **2010**, 132, 041103.

(S10) Cleland, D. M.; Booth, G. H.; Alavi, A. A Study of Electron Affinities Using the Initiator Approach to Full Configuration Interaction Quantum Monte Carlo. J. Chem. Phys. **2011**, 134, 024112.

(S11) Tubman, N. M.; Lee, J.; Takeshita, T. Y.; Head-Gordon, M.; Whaley, K. B. A Deterministic Alternative to the Full Configuration Interaction Quantum Monte Carlo Method. J. Chem. Phys. **2016**, 145, 044112.

(S12) Tubman, N. M.; Levine, D. S.; Hait, D.; Head-Gordon, M.; Whaley, K. B. An Efficient Deterministic Perturbation Theory for Selected Configuration Interaction Methods. 2018; arXiv:1808.02049.

(S13) Tubman, N. M.; Freeman, C. D.; Levine, D. S.; Hait, D.; Head-Gordon, M.; Whaley, K. B. Modern Approaches to Exact Diagonalization and Selected Configuration Interaction with the Adaptive Sampling CI Method. J. Chem. Theory Comput. **2020**, 16, 2139.

(S14) Sharma, S.; Holmes, A. A.; Jeanmairet, G.; Alavi, A.; Umrigar, C. J. Semistochastic Heat-Bath Configuration Interaction Method: Selected Configuration Interaction with Semistochastic Perturbation Theory. J. Chem. Theory Comput. **2017**, 13, 1595.

(S15) Holmes, A. A.; Umrigar, C. J.; Sharma, S. Excited States Using Semistochastic Heat-Bath Configuration Interaction. J. Chem. Phys. **2017**, 147, 164111.

(S16) Li, J.; Otten, M.; Holmes, A. A.; Sharma, S.; Umrigar, C. J. Fast Semistochastic Heat-Bath Configuration Interaction. J. Chem. Phys. **2018**, 149, 214110.

(S17) Liu, W.; Hoffmann, M. R. SDS: The 'Static–Dynamic–Static' Framework for Strongly Correlated Electrons. Theor. Chem. Acc. **2014**, 133, 1481.

(S18) Liu, W.; Hoffmann, M. R. iCI: Iterative CI toward Full CI. J. Chem. Theory Comput. **2016**, 12, 1169.

(S19) Zhang, N.; Liu, W.; Hoffmann, M. R. Iterative Configuration Interaction with Selection. J. Chem. Theory Comput. **2020**, 16, 2296.

(S20) Zhang, N.; Liu, W.; Hoffmann, M. R. Further Development of iCIPT2 for Strongly Correlated Electrons. J. Chem. Theory Comput. **2021**, 17, 949.

(S21) Ghanem, K.; Lozovoi, A. Y.; Alavi, A. Unbiasing the Initiator Approximation in Full Configuration Interaction Quantum Monte Carlo. J. Chem. Phys. **2019**, 151.

(S22) Deustua, J. E.; Shen, J.; Piecuch, P. Converging High-Level Coupled-Cluster Energetics by Monte Carlo Sampling and Moment Expansions. Phys. Rev. Lett. **2017**, 119, 223003.

(S23) Deustua, J. E.; Magoulas, I.; Shen, J.; Piecuch, P. Communication: Approaching Exact Quantum Chemistry by Cluster Analysis of Full Configuration Interaction Quantum Monte Carlo Wave Functions. J. Chem. Phys. **2018**, 149, 151101.

(S24) Deustua, J. E.; Yuwono, S. H.; Shen, J.; Piecuch, P. Accurate Excited-State Energetics by a Combination of Monte Carlo Sampling and Equation-Of-Motion Coupled-Cluster Computations. J. Chem. Phys. **2019**, 150, 111101.

(S25) Yuwono, S. H.; Chakraborty, A.; Emiliano Deustua, J.; Shen, J.; Piecuch, P. Accelerating Convergence of Equation-Of-Motion Coupled-Cluster Computations Using the Semi-Stochastic CC($P$;$Q$) Formalism. Mol. Phys. **2020**, 118, e1817592.

(S26) White, S. R. Density Matrix Formulation for Quantum Renormalization Groups. Phys. Rev. Lett. **1992**, 69, 2863.

(S27) White, S. R. Density-Matrix Algorithms for Quantum Renormalization Groups. Phys. Rev. B **1993**, 48, 10345.

(S28) White, S. R.; Martin, R. L. *Ab Initio* Quantum Chemistry Using the Density Matrix Renormalization Group. J. Chem. Phys. **1999**, 110, 4127.

(S29) Mitrushenkov, A. O.; Fano, G.; Ortolani, F.; Linguerri, R.; Palmieri, P. Quantum Chemistry Using the Density Matrix Renormalization Group. J. Chem. Phys. **2001**, 115, 6815.

(S30) Chan, G. K.-L.; Head-Gordon, M. Highly Correlated Calculations with a Polynomial Cost Algorithm: A Study of the Density Matrix Renormalization Group. J. Chem. Phys. **2002**, 116, 4462.

(S31) Legeza, O.; Röder, J.; Hess, B. A. Controlling the Accuracy of the Density-Matrix Renormalization-Group Method: The Dynamical Block State Selection Approach. Phys. Rev. B **2003**, 67, 125114.

(S32) Chan, G. K.-L.; Sharma, S. The Density Matrix Renormalization Group in Quantum Chemistry. Annu. Rev. Phys. Chem. **2011**, 62, 465.

(S33) Sharma, S.; Chan, G. K.-L. Spin-Adapted Density Matrix Renormalization Group Algorithms for Quantum Chemistry. J. Chem. Phys. **2012**, 136, 124121.

(S34) Wouters, S.; Neck, D. V. The Density Matrix Renormalization Group for Ab Initio Quantum Chemistry. Eur. Phys. J. D **2014**, 68, 272.

(S35) Olivares-Amaya, R.; Hu, W.; Nakatani, N.; Sharma, S.; Yang, J.; Chan, G. K.-L. The *Ab-Initio* Density Matrix Renormalization Group in Practice. J. Chem. Phys. **2015**, 142, 034102.

(S36) Knecht, S.; Hedegård, E. D.; Keller, S.; Kovyrshin, A.; Ma, Y.; Muolo, A.; Stein, C. J.; Reiher, M. New Approaches for *Ab Initio* Calculations of Molecules with Strong Electron Correlation. Chimia **2016**, 70, 244.

(S37) Eriksen, J. J.; Lipparini, F.; Gauss, J. Virtual Orbital Many-Body Expansions: A Possible Route Towards the Full Configuration Interaction Limit. J. Phys. Chem. Lett. **2017**, 8, 4633.

(S38) Eriksen, J. J.; Gauss, J. Many-Body Expanded Full Configuration Interaction. I. Weakly Correlated Regime. J. Chem. Theory Comput. **2018**, 14, 5180.

(S39) Eriksen, J. J.; Gauss, J. Many-Body Expanded Full Configuration Interaction. II. Strongly Correlated Regime. J. Chem. Theory Comput. **2019**, 15, 4873.

(S40) Eriksen, J. J.; Gauss, J. Generalized Many-Body Expanded Full Configuration Interaction Theory. J. Phys. Chem. Lett. **2019**, 10, 7910.

(S41) Eriksen, J. J.; Gauss, J. Ground and Excited State First-Order Properties in Many-Body Expanded Full Configuration Interaction Theory. J. Chem. Phys. **2020**, 153, 154107.

(S42) Eriksen, J. J.; Gauss, J. Incremental Treatments of the Full Configuration Interaction Problem. Wiley Interdiscip. Rev.: Comput. Mol. Sci. **2021**, 11, e1525.

(S43) Greiner, J.; Gauss, J.; Eriksen, J. J. Error Control and Automatic Detection of Reference Active Spaces in Many-Body Expanded Full Configuration Interaction. 2024; arXiv:2406.11343.

(S44) Xu, E.; Uejima, M.; Ten-no, S. L. Full Coupled-Cluster Reduction for Accurate Description of Strong Electron Correlation. Phys. Rev. Lett. **2018**, 121, 113001.

(S45) Xu, E.; Uejima, M.; Ten-no, S. L. Towards Near-Exact Solutions of Molecular Electronic Structure: Full Coupled-Cluster Reduction with a Second-Order Perturbative Correction. J. Phys. Chem. Lett. **2020**, 11, 9775.

(S46) Blankenbecler, R.; Scalapino, D. J.; Sugar, R. L. Monte Carlo Calculations of Coupled Boson-Fermion Systems. I. Phys. Rev. D **1981**, 24, 2278.

(S47) Sugiyama, G.; Koonin, S. Auxiliary Field Monte-Carlo for Quantum Many-Body Ground States. Ann. Phys. **1986**, 168, 1.

(S48) Lang, G. H.; Johnson, C. W.; Koonin, S. E.; Ormand, W. E. Monte Carlo Evaluation of Path Integrals for the Nuclear Shell Model. Phys. Rev. C **1993**, 48, 1518.

(S49) Rom, N.; Charutz, D.; Neuhauser, D. Shifted-Contour Auxiliary-Field Monte Carlo: Circumventing the Sign Difficulty for Electronic-Structure Calculations. Chem. Phys. Lett. **1997**, 270, 382.

(S50) Zhang, S.; Carlson, J.; Gubernatis, J. E. Constrained Path Monte Carlo Method for Fermion Ground States. Phys. Rev. B **1997**, 55, 7464.

(S51) Jacobi, S.; Baer, R. The Well-Tempered Auxiliary-Field Monte Carlo. J. Chem. Phys. **2003**, 120, 43.

(S52) Al-Saidi, W. A.; Zhang, S.; Krakauer, H. Auxiliary-Field Quantum Monte Carlo Calculations of Molecular Systems with a Gaussian Basis. J. Chem. Phys. **2006**, 124, 224101.

(S53) Huron, B.; Malrieu, J. P.; Rancurel, P. Iterative Perturbation Calculations of Ground and Excited State Energies from Multiconfigurational Zeroth-Order Wavefunctions. J. Chem. Phys. **1973**, 58, 5745.

(S54) Evangelisti, S.; Daudey, J.-P.; Malrieu, J.-P. Convergence of an Improved CIPSI Algorithm. Chem. Phys. **1983**, 75, 91.

(S55) Cimiraglia, R.; Persico, M. Recent Advances in Multireference Second Order Perturbation CI: The CIPSI Method Revisited. J. Comput. Chem. **1987**, 8, 39.

(S56) Zimmerman, P. M. Incremental Full Configuration Interaction. J. Chem. Phys. **2017**, 146, 104102.

(S57) Zimmerman, P. M. Singlet–Triplet Gaps through Incremental Full Configuration Interaction. J. Phys. Chem. A **2017**, 121, 4712.

(S58) Zimmerman, P. M. Strong Correlation in Incremental Full Configuration Interaction. J. Chem. Phys. **2017**, 146, 224104.

(S59) Rask, A. E.; Zimmerman, P. M. Toward Full Configuration Interaction for Transition-Metal Complexes. J. Phys. Chem. A **2021**, 125, 1598.

(S60) Greiner, J.; Eriksen, J. J. `PyMBE`: A Many-Body Expanded Correlation Code. See: `https://gitlab.com/januseriksen/pymbe`.

(S61) Hoefler, T.; Dinan, J.; Buntinas, D.; Balaji, P.; Barrett, B.; Brightwell, R.; Gropp, W.; Kale, V.; Thakur, R. MPI+MPI: A New Hybrid Approach to Parallel Programming with MPI Plus Shared Memory. Computing **2013**, 95, 1121.

(S62) Eriksen, J. J.; Anderson, T. A.; Deustua, J. E.; Ghanem, K.; Hait, D.; Hoffmann, M. R.; Lee, S.; Levine, D. S.; Magoulas, I.; Shen, J.; Tubman, N. M.; Whaley, K. B.; Xu, E.; Yao, Y.; Zhang, N.; Alavi, A.; Chan, G. K.-L.; Head-Gordon, M.; Liu, W.; Piecuch, P.; Sharma, S.; Ten-no, S. L.; Umrigar, C. J.; Gauss, J. The Ground State Electronic Energy of Benzene. J. Phys. Chem. Lett. **2020**, 11, 8922.
